# Supplementary material for: Anthropomorphic tissue-mimicking phantoms for oximetry validation in multispectral optical imaging
Source: arXiv:2503.23161 source file (2025-03-29)
Supplement: Supplementary file 1 [file Baseline_BXX_Multispectral_Phantoms.pdf]

# Measurement Protocol for Multispectral Photoacoustic Inclusion Materials

**Date:** ______________________

**Operator:** ______________________

**Experiment ID:** ______________________

**Colour:** ______________________

## Phantom preparation protocol

Please check the boxes when a step has been finished!

### ☐ Step 1: Prepare 30 ml stock solution with 2 mg/ml

| Check? | Instruction | Comment | |
|---|---|---|---|
| ☐ | Weigh 30 ml (25.14 g) of mineral oil in a skirted tube | $M_{measured}$: | g |
| ☐ | Weigh 60 mg of the dye powder | $M_{measured}$: | mg |
| ☐ | Mix the mineral oil and the dye in the vortexer (30 s) | $T_{vortexed}$: | s |
| ☐ | Sonicate in the water bath sonicator for 10 s and then shake the tube by hand. (repeat ~10 times) | $N_{repetitions}$: | |
| ☐ | Crush the little bits and clumps of the dye with a spatula. | | |
| ☐ | Repeat the previous 3 steps until there are no clumps left that are bigger than a granule of sugar. | | |
| ☐ | Label the tube with the dye ID and the date of production | | |

### ☐ Step 2: Prepare phantoms according to multicentre study

The following steps are meant to briefly summarise and amend the IPASC multicenter phantom material verification study 2022 Protocol. This means that the steps are adjusted to a 50 ml volume of mineral oil (conversion ratio of 0.5 from 100 ml to 50 ml). In doubt, please refer to the full study protocol!

| Check? | Instruction | Comment | |
|---|---|---|---|
| ☐ | Prepare a silicone oil bath, set the temperature to 160°C | | |
| ☐ | Weigh 50 ml (41.90 g) of mineral oil in a beaker (beaker 1) | $M_{measured}$: | g |

| | | | |
|---|---|---|---|
| ☐ | Vortex the stock solution for 1 min | $T_{vortexed}$: | min |
| ☐ | Pipette 12.8 ml of the stock solution | Stock solution: | |
| ☐ | Add the stock solution to beaker 1 | | |
| ☐ | Weigh 76.5 mg of TiO2 and add to beaker 1 | $M_{measured}$: | mg |
| ☐ | Sonicate and sway beaker 1 until no TiO2 is settled at the bottom. This will take roughly 20 - 30 min. In the meantime, the following 3 steps can be performed. | $T_{sonicated}$: | min |
| ☐ | Weigh 1.0 g of Butylated Hydroxytoluene | $M_{measured}$: | g |
| ☐ | Weigh 12.57 g of SEBS | $M_{measured}$: | g |
| ☐ | Add SEBS and Butylated Hydroxytoluene with a magnet stirrer in a new beaker (beaker 2) | | |
| ☐ | When there is no settled TiO2 left in beaker 1, pour the content of beaker 1 into beaker 2 | | |
| ☐ | Heat beaker 2 in the oil bath for about 45 min with aluminium foil on top | $T_{in\ oil}$: | min |
| ☐ | After 10 min, take off the aluminium cover and stir the mixture with a metallic spoon/spatula. | | |
| ☐ | When the mixture has become liquid, put in vacuum chamber for at least 1 min | $T_{in\ vacuum}$: | min |
| ☐ | Scratch residual bubbles from surface and repeat the previous step if necessary | | |

## ☐ Step 3: Casting the phantom material into the mold for optical samples

This step is for fabricating the optical samples used to measure absorption and scattering of the material. For this, take four microscopy glass slides, put a metallic frame on two of the slides and pour the material in it. Try to be quick when covering the material and the metallic frame so that the material is still fluid and can be compressed into shape.
